# Supplementary material for: Review-driven Personalized Preference Reasoning with Large Language Models for Recommendation
Source: arXiv:2408.06276 source file (2025-04-25)
Supplement: Supplementary file 1 [file 049CaseStudyForAppendix.tex]

Table \ref{tbl:casestudyforappendix} present explanation generated for user /user/ur18123905/ and item 2084970 : The Imitation Game (2014) generated by \proposed.

\begin{table*}[t]
\centering
% \small
\caption{Explanations generated by LLM-based models}
% \resizebox{0.99\linewidth}{!}{
\begin{tabular}{P}
\toprule
\textbf{UserID}: /user/ur18123905/, \textbf{ItemID}: 2084970 \\\midrule
\textbf{Item Title}: The Imitation Game (2014) \\
\textbf{Item Genres}: Biography, Drama, Thriller, War\\
\textbf{Item Directors}: Morten Tyldum\\
\textbf{Item Cast}: Benedict Cumberbatch, Keira Knightley, Matthew Goode\\
\textbf{Item Plot}: It is based on the real life story of legendary cryptanalyst Alan Turing. The film portrays the nail-biting race against time by Turing and his brilliant team of code-breakers at Britain's top-secret Government Code and Cypher School at Bletchley Park, during the darkest days of World War II. \\\vspace{5pt}
\textbf{User Profile} (by \proposed): \\
{[\textit{Like}]}\\
- Appreciates visually stunning cinematography\\
- Enjoys strong and memorable storytelling\\
- Values chemistry and relationships between characters\\
- Enjoys thought-provoking and intense films\\
- Appreciates fresh and unique concepts\\
{[\textit{Dislike}]}\\
- Dislikes predictability and cliches in movies\\
- Prefers relatable and likable protagonists\\
- Dislikes forced or unnatural dialogue\\
- Dislikes prolonged or unnecessary scenes\\
- Dislikes lack of focus or transparency in storytelling\\\vspace{5pt}
\textbf{Item Profile} (by \proposed): \\
{[\textit{Like}]}\\
- Benedict Cumberbatch's performance was frequently highlighted as exceptional.\\
- The portrayal and exploration of Alan Turing's personal and professional life.\\
- Historical significance and educational value regarding Turing's contributions during WWII.\\
- High-quality acting from the supporting cast, including Keira Knightley and Matthew Goode.\\
- Well-crafted storytelling and direction, emphasizing the dramatic and emotional aspects of Turing's story.\\
{[\textit{Dislike}]}\\
- Excessive focus on Turing's personal life at the expense of other story elements.\\
- Some viewers criticized the film for taking liberties with historical facts.\\
- Use of flashbacks and non-linear storytelling was not appreciated by all.\\
- Perceived as playing it too safe or vague in dealing with sensitive historical issues.\\
- Criticisms of other technical aspects like editing, soundtrack, and some supporting performances.
\\
\midrule
\textbf{Generated Explanations} \\ \midrule
\textbf{\pfive}: The secrets behind the true victors of World War II were only divulged not too long ago (interestingly enough, it's hard to come by the exact date of the reveal). 
\\\vspace{5pt} 
\textbf{\xrec}: You would enjoy "The Imitation Game" because it celebrates the genius of Alan Turing without sentimentally concluding that there's a genius in everyone. The film's execution, integrity in character portrayal, and the dynamic between the characters make it a compelling and emotionally impactful watch.
\\\vspace{5pt}
\textbf{\proposed}: The user would likely enjoy "The Imitation Game" as it offers visually stunning cinematography and a strong, memorable storytelling. The film delves into the personal and professional life of Alan Turing, providing a thought-provoking and intense narrative. The chemistry and relationships between characters, particularly Benedict Cumberbatch's exceptional performance, would be appreciated by the user. Additionally, the historical significance and educational value regarding Turing's contributions during WWII align with the user's preference for fresh and unique concepts. However, the excessive focus on Turing's personal life and the film's perceived vagueness in dealing with sensitive historical issues may be points of contention for the user. Nonetheless, the overall quality of acting and well-crafted storytelling would likely make "The Imitation Game" a recommended watch for the user.
\\ \bottomrule
\end{tabular}
% }
% \vspace{0.2cm}
\label{tbl:casestudyforappendix}
\end{table*}
