# Supplementary material for: Review-driven Personalized Preference Reasoning with Large Language Models for Recommendation
Source: arXiv:2408.06276 source file (2025-04-25)
Supplement: Supplementary file 2 [file 048ComponentAnalysis_additional.tex]

To validate the performance using different LLM, we use the same prompts provided to \proposed, which corresponds to the third method in Table \ref{tbl:no_bias_reasoning}, but employing GPT-4 instead of GPT-3.5.
The result in Table \ref{tbl:no_bias_reasoning_additional} supports the necessity of fine-tuning in the recommendation domain and shows that knowledge distillation process improves a smaller LLM, enhancing both cost-efficiency and recommendation accuracy.
% While GPT-4 offers advanced capabilities, we choose GPT-3.5 as the teacher LLM for its ability to generate high-quality labeled data at a substantially lower computational cost, ensuring a balance between efficiency and effectiveness.

\begin{table}[H]
\centering
\caption{Validation with different LLM (*: $p$-value < 0.05).}
\label{tbl:no_bias_reasoning_additional}
\resizebox{0.99\linewidth}{!}{
\begin{tabular}{cccQQQQ}
\toprule
\multirow{2.5}{*}{\textbf{Methods}} & \multirow{2.5}{*}{\textbf{R}} & \multirow{2.5}{*}{\textbf{B}} & \multicolumn{2}{c}{\textbf{IMDB}} & \multicolumn{2}{c}{\textbf{Amazon-book}} \\ \cmidrule(lr){4-5}\cmidrule(lr){6-7}
& & & \textbf{RMSE} & \textbf{MAE} & \textbf{RMSE} & \textbf{MAE} \\ \midrule
% \gptfour & \cmark & \cmark & 2.0688 & 1.6489 & 0.9038 & 0.6518 \\ \midrule
{\shortstack{\gptfour, ZS}} & \cmark & \cmark & 2.0628 & 1.5769 & 0.9120 & 0.5788 \\ \midrule

% \gptthree & \cmark & \cmark & 2.0688 & 1.6489 & 0.9038 & 0.6518 \\ \midrule
{\shortstack{\gptthree, ZS}} & \cmark & \cmark & 2.0688 & 1.6489 & 0.9038 & 0.6518 \\ \midrule

\proposed & \cmark & \cmark & \textbf{1.9122}* & \textbf{1.4691}* & \textbf{0.6508}* & \textbf{0.4297}* \\ \bottomrule
\end{tabular}
}
\end{table}
